# Supplementary material for: New Results on a General Class of Minimum Norm Optimization Problems
Source: arXiv:2504.13489 source file (2025-04-30)
Supplement: Supplementary file 3 [file appendix-5-backup.tex]

\section{Algorithms and Proofs Omitted in Section 5}
\subsection{An Overview of Our Algorithm}
We can write down the following natural linear programming formulation for the \LBO\ version:

\begin{equation}
\begin{aligned}
	\min && 0 && & \\
    s.t. && \sum_{v\in \calU} x_v w_{v,i}\geq 1 && & \forall 1\leq i\leq d\\
    && \sum_{v\in S_j} x_v\leq 2^j && & \forall 1\leq j\leq T\\
    && 0\leq x_v\leq 1 && & \forall v\in S_j,1\leq j\leq T
\end{aligned}
\tag{LP-KnapCover-1}
\label{LP-KnapCover-1}
\end{equation}

Our goal is to find an integer solution $\{x_v\}_{v\in\calU}$ such that
\begin{equation}
\begin{aligned}
    && \sum_{v\in \calU} x_v w_{v,i}\geq 1 && & \forall 1\leq i\leq d\\
    && \sum_{v\in S_j} x_v\leq c\times 2^j && & \forall 1\leq j\leq T\\
    && 0\leq x_v\leq 1 && & \forall v\in S_j,1\leq j\leq T
\end{aligned}
\end{equation}

for some constant $c$.

We give two algorithms in this section. In \autoref{sec:Knap-1}, we present an algorithm that solves the $2$-\LBO\ $d$-dimensional knapsack cover problem in polynomial time for $d = O(1)$. For the second algorithm, we introduce a new quantity, $W$, representing the maximum ratio between the maximum weight and the minimum non-zero weight across all dimensions. The second algorithm can solve the same problem (the $2$-\LBOknapcov\ ) in polynomial time when $d = O\left(\sqrt{\frac{\log n}{\log\log W}}\right)$. This result indicates that if $W$ can be bounded by a polynomial in $n$, $d$ can be significantly larger than a constant.

In the first algorithm, we partially enumerate the items chosen in the first $T_0=\lceil \log d \rceil$ sets (the partial enumeration is defined in section 5.3) and then attempt to add items in sets $S_{T_0+1}, S_{T_0+2}, \ldots, S_{T}$. Since $d$ is a constant, we can ensure the enumeration is polynomial time. The enumeration outputs a series of \textbf{partial solution}s, and a \textbf{partial solution} can be described as a vector $(D_1,D_2,\cdots, D_{T_0})$, where $D_i\subseteq S_i$ for $i=1,2,\cdots, T_0$. After that, We sequentially enumerate these partial solutions. For each partial solution, we use it to modify the Linear Programming (\ref{LP-KnapCover-1}) and perform iterative rounding. For each iteration of the iterative rounding, we find an extreme point and change the form of the Linear Programming. Ultimately, we obtain a $2$-valid solution or ensure no $1$-valid solution for this enumeration result. 

The second algorithm uses the same iterative rounding method but changes the enumeration step. We use a technique called \textbf{partial enumeration} instead of listing all partial solutions. Partial enumeration lists a subset of all possible partial solutions for the first several sets. We ensure the partial enumeration algorithm is polynomial time and the iterative rounding can still find a good solution based on at least one partial solution in the subset output by the algorithm. The details are shown in \autoref{sec:Knap-2}.      


\subsection{An Algorithm for $d=O(1)$} \label{sec:Knap-1}

In this subsection, we assume that $d$ is a constant and present a polynomial-time algorithm to solve the $2$-\LBOknapcov\ (the time complexity is $O(n^{4d})$). Thus, we can design a constant approximation factor algorithm for the \minnormknapcov\ .

In this subsection, we use an iterative rounding algorithm. We maintain a integer variable $\beta$ and iteratively focus on the first beta sets ($S_1,S_2,\cdots ,S_{\beta}$). Since the rounding algorithm does not work when $\beta\le \log d$, we define $T_0=\lceil \log d\rceil$ and incorporate an additional component in the algorithm to handle this case.  

Specifically, for a vector $t \in \mathbb{R}^d$ and a non-negative integer $\beta \leq T$, we concentrate on the following linear program:

\begin{equation}
\begin{aligned}
    \min \quad & 0 \\
    \text{s.t.} \quad & \sum_{T_0 < j \leq \beta} \sum_{u \in S_j} x_u w_{u,i} \geq t_i \quad & \forall 1 \leq i \leq d, \\
    & \sum_{u \in S_j} x_u \leq 2^j \quad & \forall T_0 < j \leq \beta, \\
    & 0 \leq x_u \leq 1 \quad & \forall u \in S_j, \; T_0 < j \leq \beta.
\end{aligned}
\tag{LP-KnapCover($t$, $\beta$)}
\label{LP-KnapCover}
\end{equation}

First we present the entire algorithm. Initially, let $\beta = \lceil \log n \rceil$. First, we enumerate the first $T_0$ sets to find all partial solutions $D_1, D_2, \dots, D_{T_0}$ that satisfy:

- $|D_i| \leq 2^i$ for $i = 1, 2, \dots, T_0$.

Then we need to construct $D_{T_0+1},D_{T_0+2},\cdots,D_T$.
For a partial solution $(D_1, D_2, \dots, D_{T_0})$, a solution $D \subseteq \calU$ is called an \textbf{Extended Solution} of $(D_1, D_2, \dots, D_{T_0})$ if and only if:

\[
D \cap S_j = D_j \quad \text{for each } 1 \leq j \leq T_0.
\]
Without loss of generality, we sometimes describe the Extended Solution in the form of $D_1, D_2, D_3, \dots, D_T$. 

After the enumeration, we sequentially check these partial solutions. For each partial solution, we initialize:

\[
t_i = 1 - \sum_{j=1}^{T_0} \sum_{u \in D_j} w_{u,i}.
\]

Next, we start iterative rounding until $\beta \leq T_0$. At each iteration, we solve the LP (\ref{LP-KnapCover}) and perform the following steps:

\begin{enumerate}
    \item Check the Linear Programming (\ref{LP-KnapCover}). If there is no solution, then return "No Solution" directly. Otherwise, obtain an extreme point $x^{*}$ for (\ref{LP-KnapCover}).

    \item For any $T_0< j\leq \beta+d$ such that $2^j > \beta + d$ (i.e. $j> \log (\beta+d)$), round the non-integer $x^{*}_u$ values to 1 for all $u \in S_j$. More specifically, we add them to our extended solution: $D_j \gets \{u \in S_j : x^{*}_u > 0\}$ for all $j$ such that $T_0 < j \leq \beta$ and $2^j > \beta + d$.

    \item Update $t_i$ by subtracting the weights of the newly added items.

    \item Update $\beta$ to $\lfloor \log (\beta + d) \rfloor$.
\end{enumerate}

\begin{algorithm}
\caption{Iterative Rounding for $d$-dimension Knapsack Cover Problem} \label{Algo-IR-Knap}
\KwResult{Solution $D$ or "No Solution"}
$\beta \gets T$\;
$D \gets D_1 \cup D_2 \cup \dots \cup D_{T_0}$\;
$t_i \gets 1 - \sum_{j=1}^{T_0} \sum_{u \in D_j} w_{u,i}$ for each $1 \leq i \leq d$\;
\While{$\beta > T_0$}{
    \If{LP-KnapCover($t$, $\beta$) has no solution}{
        Return "No Solution"\;
    }
    Solve Linear Programming LP-KnapCover($t$, $\beta$) and obtain an extreme point $x^{*}$\;
    $D \gets D \cup \{u \in S_j \mid T_0 < j \leq \beta, 2^j > \beta + d, x^{*}_u > 0\}$\;
    $t_i \gets t_i - \sum_{T_0 < j \leq \beta : 2^j > \beta + d} \sum_{u \in S_j : x^{*}_u > 0} w_{u,i}$ for all $1 \leq i \leq d$;
    $\beta \gets \lfloor \log (\beta + d) \rfloor$\;
}
Return $D$\;
\end{algorithm}


\begin{lemma} \label{lem:Knap-1}
If $d > 1$, the loop of the iterative rounding (lines 3 to 9) can definitely terminate, and it takes $O(\log^{*} n)$ iterations. ($\log^* n$ represents the number of times you need to iteratively apply the logarithm function to a number 
$n$ until the result is less than or equal to a fixed constant)
\end{lemma}
\begin{proof}
We discuss the two cases:

\begin{enumerate}
\item $\beta > 3d$: We notice that 
$$\lfloor \log(\lfloor \log(\beta + d) \rfloor + d) \rfloor\leq \log\left(\frac{\beta+d}{2} + d\right) < \log \beta$$ for any $\beta > d > 1$.
The first inequality is based on the fact that when $x\geq 5$, we have $\frac{x}{2}>\log x$.
So for $\beta>3d$, $O(\log^{*} n)$ iterations can change $\beta$ to a number at most $3d$.

\item $1+\log d \leq \beta \leq 3d$: We have 
$$\log(\beta + d)\leq \log (\beta+2^{\beta-1}) <\log (2^{\beta-1}+2^{\beta-1})= \beta$$ for any $d > 1$ and $\beta \geq 1+\log d$. Thus, $\beta$ decreases by at least 1 in each subsequent iteration. Therefore, it takes a constant number of iterations until $\beta$ becomes at most $\lceil \log d\rceil$.
\end{enumerate}

Overall, after $O(\log^{*} n)$ iterations, the loop must terminate.
\end{proof}

\begin{lemma} \label{lem:Knap-2}
If $d > 1$, there exists an $O(n^{4d})$-time algorithm to enumerate all partial solutions $(D_1, \cdots, D_{T_0})$ satisfying $|D_i| \le 2^i$ for all $1 \le i \le T_0$($T_0=\lceil \log d\rceil$). 
\end{lemma}
\begin{proof}
Assume that $n\geq 4d$ as $d$ is a constant. We need to select at most $2^i$ items from $S_i$ for $1\leq i\leq T_0$. So $2^i\leq 2^{\log d+1}=2d<n/2$. The number of ways to choose these items is not greater than: 
\[
\sum_{j=0}^{2^i} \binom{|S_i|}{j} \leq \sum_{j=0}^{2^i} \binom{n}{j}\leq (2^i+1)\binom{n}{2^i}\leq (2^i+1)\cdot\frac{n^{2^i}}{(2^i)!}.
\]
It is at most $n^{2^i}$ when $i\geq 2$. When $i=1$, as $n\geq 4$,
\[
\sum_{j=0}^{2^i} \binom{|S_i|}{j} \leq \sum_{j=0}^{2^i} \binom{n}{j}=1+n+\frac{n(n-1)}{2}\leq n^2.
\]
Therefore, the total number of those partial solutions is no more than:
\[
\prod_{i=1}^{\lceil \log d \rceil} n^{2^i} = n^{\sum_{i=0}^{\lceil \log d \rceil} 2^i} \le n^{2^{2+\log d}} = O(n^{4d})
\]

Those formulas can be also associated with a simple brute force algorithm, thus the total complexity is $O(n^{4d})$.
\end{proof}

\begin{lemma} \label{lem:Knap-3}
If the iterative rounding (Algorithm \ref{Algo-IR-Knap}) returns a solution $D$, then $|D \cap S_j| \le 2^{j+1}$ for all $1 \le j \le T$.
\end{lemma}
\begin{proof}

\emph{Case 1}: $j \le \lceil \log d \rceil$. In this case, $D \cap S_j = D_j$ and it must satisfy the condition.

\emph{Case 2}: $j > \lceil \log d \rceil$. For such a $j$, $|D \cap S_j|$ is determined by an iteration starting with parameter $\beta$, where $\lfloor \log(\beta + d) \rfloor < j \le \beta$. 

Let $x^{*}$ be the extreme point in this iteration. By Lemma~\ref{lem:extreme:points}, if $x^*$ has $m$ dimensions, then there are $m$ linearly independent constraints of \ref{LP-KnapCover} that hold with equality at $x^*$.
If the basis contains equality $x_u = 0$ or $x_u = 1$ for some $u \in S_j$, then $x^{*}_u$ must be an integer. The number of other constraints is exactly $\beta -T_0 + d$, so the number of non-integer $x^{*}_u$ is at most $\beta - T_0 + d \le \beta + d$. Therefore,

\[
|D \cap S_j| = \sum_{u \in S_j} \mathbf{1}_{x^{*}_u > 0} \le \left( \sum_{u \in S_j} \mathbf{1}_{0 < x^{*}_u < 1} \right) + \left( \sum_{u \in S_j} x^{*}_u \right) \le \beta + d + 2^j \le 2^{j+1}.
\]
\end{proof}

\begin{lemma} \label{lem:Knap-4}
If (\ref{LP-KnapCover-1}) has an integral solution, then there exists an enumeration result $D_1, \cdots, D_{T_0}$ such that Algorithm \ref{Algo-IR-Knap} finds an extended solution.
\end{lemma}
\begin{proof}

Since (\ref{LP-KnapCover-1}) has an integral solution, there exists $D_1, D_2, \cdots, D_{T_0}$ such that the LP in the first iteration of Algorithm \ref{Algo-IR-Knap} has a non-empty solution set. If the $i$-th iteration of Algorithm \ref{Algo-IR-Knap} does not return "No Solution", then the fractional solution $x^{*}$ corresponds to a feasible solution for the LP in the $(i+1)$-th iteration. Therefore, if the first iteration does not return "No Solution", the algorithm never returns "No Solution". By the existence of integral solution, the algorithm doesn't return "No Solution" in the first iteration.

\end{proof}

\begin{proofofthm}{\ref{thm:knap-1}}
This theorem can be proven by the combination of the following results obtained from the previous lemmas.

- The enumeration complexity is $O(n^{4d}) = poly(n)$ (Lemma \ref{lem:Knap-2}).

- The iterative rounding takes polynomial time (Lemma \ref{lem:Knap-1}, Lemma \ref{lem:Knap-4}).

Therefore, Algorithm \ref{Algo-IR-Knap} terminates in polynomial time. Moreover, according to Lemmas \ref{lem:Knap-3} and \ref{lem:Knap-4}, it returns a $2$-valid solution or confirms that there is no $1$-valid solution.

\end{proofofthm}
\subsection{An Algorithm for \(d = O\left( \sqrt{\frac{\log n}{\log\log W}}\right)\)} \label{sec:Knap-2}

In this subsection, we focus on the case of larger \(d\). We can notice that the bottleneck of our previous algorithm is the Enumeration Algorithm with \(O(n^{4d})\) time complexity. Similarly, we denote \(T_0 = \lceil \log d \rceil\). Here we first generalize the previous enumeration algorithm discussed in \autoref{sec:Knap-1}, and call the generalized technique as \textbf{partial enumeration}.

\begin{definition}[Partial Enumeration] \label{def:part-enum}
For a $(c,c_0)$-\LBO\ problem with set $S_1,S_2,\cdots S_{T}$, a \textbf{partial enumeration} algorithm has a quantity $T_0$ based on the $(c,c_0)$-\LBO\ problem. The partial enumeration algorithm returns a subset $X\subseteq 2^{S_0}\times 2^{S_1}\times \cdots \times 2^{S_{T_0}}$. Each element of this subset is a \textbf{partial solution} $(D_1,D_2,\cdots D_{T_0})$(Recall the definition of partial solution: $D_i\subseteq S_i$), and this algorithm ensures: 

\begin{enumerate}
    \item If there exists a $c_0$-valid solution, then at least one partial solution $(D_1,D_2,\cdots D_{T_0})\in X$ satisfy there exists an $c$-valid \textbf{extended solution} (Recall, a solution $D$ is called an extended solution if $D\cap S_i=D_i$ for all $i=1,2,\cdots, T_0$).

    \item The size of output, $X$, is polynomial size, and this partial enumeration algorithm is always polynomial time.
\end{enumerate}
\end{definition}

Recall that we define $W=\max_{1\le i\le d} \frac{\max_{u\in \calU} w_{u,i}}{\min_{u\in \calU,w_{u,i}>0} w_{u,i}}$.
%For an arbitrary coordinate $i$ and a set $S$, we define the weight gap as:

%$$\wgap(S,i)=\left\lbrace \begin{aligned}
%    & 0 && \text{if }\forall u\in S,w_{u,i}>0\\
%    &\frac{\max_{u\in S} w_{u,i}}{\min_{u\in S,w_{u,i}>0} w_{u,i}} && \text{otherwise}\\
%\end{aligned}\right.
%$$

%For the whole \LBO\ problem, we define the weight gap as:

%$$\wgap=\max_{1\le j\le T,1\le i\le d} \wgap(S_j,i).$$  

In this section, we use the partial enumeration method to give an algorithm for  \(d = O\left(\sqrt{\frac{\log n}{\log\log W}}\right)\).

Here is the overview of the algorithm for the \LBOknapcov\ . We first use a partial enumeration algorithm.  In the partial enumeration algorithm, we first obtain a set $X_j\subseteq 2^{S_j}$ for each \(1 \le j \le T_0\), and then combine them by direct product: \(X = X_1 \times X_2 \times \cdots \times X_{T_0}\). For each \(j\), we classify \(w_{u,i}\) into \(O(\log W)\) groups for each coordinate \(i = 1, 2, \cdots, d\), and partition \(u \in S_j\) into a total of \(O((\log W)^d)\) groups. We then enumerate the number of elements in each group and select arbitrary elements in the groups. For each partial solution \((D_1, D_2, \cdots D_{T_0}) \in X\), we use it as part of the input for Algorithm \ref{Algo-IR-Knap}, and run the iterative rounding. 

As the process after partial enumeration is the same with the previous section, we focus on the partial enumeration process. The concrete steps are shown as follows:

\begin{enumerate}
\item For each dimension \(i\), find the minimum positive weight \(\gamma_{j,i}\) among all items in \(S_j\) (if all of them are 0, \(\gamma_{j,i}\) can be anything and we do not care about it).

\item Construct a transformed vector \(w'_u\) for each \(u\) in \(S_j\):
\begin{itemize}
    \item If \(w_{u,i} > 0\), set \(w'_{u,i} = \lfloor \log(w_{u,i}/\gamma_{j,i}) \rfloor + 1\).
    \item If \(w_{u,i} = 0\), set \(w'_{u,i} = 0\).
\end{itemize}

\item Define two vectors \(w'_u\) and \(w'_v\) as equal if and only if \(w'_{u,i} = w'_{v,i}\) for all \(i = 1, 2, \cdots, d\). Calculate \(r_j\) as the number of different \(w'_u\).

\item Partition \(S_j\) into \(r_j\) sets: \(S_{j,1}, S_{j,2}, \cdots, S_{j,r_j}\) based on different \(w'_u\). Formally, for all \(u \in S_{j,x}\) and \(v \in S_{j,y}\), it should satisfy:
\[
x = y \quad \text{if and only if} \quad w'_u = w'_v.
\]

\item For each vector \(c \in \mathbb{Z}^{r_j}\) such that \(c_k \le |S_{j,k}|\) for all \(1 \le k \le r_j\) and $c_1+c_2+\cdots+c_{r_j}\leq 2^j$, construct a subset \(D'\) from \(S_j\) such that it contains exactly \(\min \{2c_k, |S_{j,k}|\}\) elements from each partition \(S_{j,k}\), and append \(D'\) to \(X_i\).
\end{enumerate}
\begin{algorithm}
\caption{Partial Enumeration Algorithm for $d$-dimensional Knapsack Cover Problem} \label{Algo-Enum-Knap}
\KwResult{a set $X$ that $X\subseteq 2^{S_1}\times \cdots \times 2^{S_{T_0}}$}
$X_i\gets \emptyset\forall i=1,\cdots d$\;
\ForAll{$j=1$ to $T_0$}{
$\gamma_{j,i}\gets \min_{u\in S_j,w_{u,i}>0}\lbrace w_{u,i}\rbrace$ for all $1\le i\le T_0$\;
Define vector $w'_u\in \mathbb{R}^{d}$ for all $u\in S_j$\;
\ForAll{$u\in S_j$, $i\in \lbrace 1,2,\cdots d\rbrace$}{
    \eIf{$w_{u,i}=0$}{
        $w'_{u,i}\gets 0$\;
    }{
        $w'_{u,i}\gets 1+\lfloor \log(w_{u,i}/\gamma_{j,i})\rfloor$\;
    }
}
Partition $S_j$ into several sets $S_{j,1},S_{j,2},\cdots S_{j,r_j}$ based on different $w'$(For $u\in S_{j,x},v\in S_{j,y}$, $w'_u=w'_v$ if and only if $x=y$)\;

\ForAll{Vector $c\in \mathbb{Z}_{\ge 0}^{r_j}$ that $c_k\le |S_{j,k}|$ for all $1\le k\le r_j$ and $c_1+c_2+\cdots+c_{r_j}\leq 2^j$} {
    Construct a subset $D'\subseteq S_j$ such that contains exactly $\min\lbrace 2c_k,|S_{j,k}|\rbrace$ elements in $S_{j,k}$\;
    $X_i\gets X_i\cup \lbrace D'\rbrace$
}
}
Return $X=X_1\times \cdots \times X_{T_0}$\;
\end{algorithm}


\begin{lemma}\label{lem:Knap-Enum-1}
\cref{Algo-Enum-Knap} is \(poly(n, \log(W))\)-time for \(d = O\left(\sqrt{\frac{\log n}{\log\log W}}\right)\).
\end{lemma}
\begin{proof}
Fix $1\leq j\leq T_0$. For an arbitrary $i$, notice that the number of different $w'_{u,i}$ ($u\in S_j$) is not larger than \(\log(W) + 2\). The number of elements in $S_i$ is no more than $d$, so we have:

\[
r_j \le (\log(W) + 2)^d = \exp(O(d \cdot \log\log(W)))
\]

To enumerate the vector \(c\) for $j$, we consider the number of non-negative integer solutions of:
$$y_1+y_2+\cdots+y_{r_j}\leq 2^j.$$
The number of solutions is well known to be
$$\binom{2^j+r_j-1}{r_j-1}=\binom{2^j+r_j-1}{2^j}\leq r_j^{2^j}.$$
Recall we just need to enumerate the first \(T_0 = \lceil \log d \rceil\) sets. Thus the total complexity is no more than:

\[
\prod_{j=1}^{T_0} r_j^{2^j} \le (\max_{j} r_j)^{2^{T_0}} = (\max_{j} r_j)^{O(d)} = \exp(O(d^2 \cdot \log\log(W)))
\]

which is \(poly(n, \log(W))\).
\end{proof}

\begin{lemma}\label{lem:Knap-Enum-Replace}
For any integer \(j, x\) and \(u_0, u_1, u_2 \in S_{j,x}\), \(w_{u_0,i} + w_{u_1,i} \ge w_{u_2,i}\) for all \(1 \le i \le d\). 
\end{lemma}
\begin{proof}
By definition, we know \(w'_{u_0,i} = w'_{u_1,i} = w'_{u_2,i}\). If \(w'_{u_0,i} = 0\), then \(w_{u_0,i} = w_{u_1,i} = w_{u_2,i} = 0\). The inequality holds. Otherwise, \(\lfloor \log(w_{u_0,i}/\gamma_{j,i}) \rfloor = \lfloor \log(w_{u_2,i}/\gamma_{j,i}) \rfloor\), then \(w_{u_0,i} \ge \frac{1}{2} w_{u_2,i}\). Similarly, \(w_{u_1,i} \ge \frac{1}{2} w_{u_2,i}\), so the inequality holds.
\end{proof}

\begin{lemma}\label{lem:Knap-Enum-2}
If the original problem has a $1$-valid solution, then there exists an enumeration result $D_1, D_2, \cdots D_{T_0}$ such that there exists an extended solution $D_1, \cdots D_T$ satisfying:
\begin{enumerate}
    \item $|D_j| \le 2 \times 2^j$ for $1 \le j \le T_0$, and 
    \item $|D_j| \le 2^j$ for $T_0 < j \le T$.
\end{enumerate}
\end{lemma}
\begin{proof}
Assume $D^{*}_1, D^{*}_2, \cdots D^{*}_T$ is a $1$-valid solution. For each $1 \le j \le T_0$, assume the enumeration process allocates $c_k = |D^{*}_j \cap S_{j,k}|$. Then $S_{j,k}$ chooses $\min \{2c_k, |S_{j,k}|\}$ elements.

- If $c_k < \frac{1}{2} |S_{j,k}|$, due to Lemma \ref{lem:Knap-Enum-Replace}, the sum of chosen weight vectors is no less than that of $S_{j,k} \cap D^{*}$ in all dimensions, and $|D_j \cap S_{j,k}| \le 2|D^{*}_j \cap S_{j,k}|$.

- Otherwise, if $c_k \ge \frac{1}{2} |S_{j,k}|$, then it selects the whole set $S_{j,k}$. The weight cannot be less, and the number of elements is also no more than $2|D^{*}_j \cap S_{j,k}|$.

Combining the two cases, we have:
\begin{enumerate}
    \item $\sum_{u \in D_j \cap S_{j,k}} w_{u,i} \ge \sum_{u \in D^{*}_j \cap S_{j,k}} w_{u,i}$ for all such $i$, and
    \item $|D_j \cap S_{j,k}| \le 2|D^{*}_j \cap S_{j,k}|$.
\end{enumerate}
Therefore, $D^{*}_1, D^{*}_2, \cdots D^{*}_{T_0}, D_{T_0+1}, \cdots D_T$ form such an extended solution satisfying those constraints.
\end{proof}

\begin{lemma}
\autoref{Algo-Enum-Knap} is a \textbf{Partial Enumeration Algorithm} for $2$-\LBO\ $d$-dimension knapsack cover problem when $d=O(\sqrt{\frac{\log n}{\log\log W}})$. More specifically, it satisfies the following properties:

\begin{enumerate}

\item If this problem has a $1$-valid solution, at least one of its output partial solutions has a $2$-valid extended solution.

\item It always runs in polynomial time.

\end{enumerate}
\end{lemma}
\begin{proof}
\cref{lem:Knap-Enum-2} implies the first property and \cref{lem:Knap-Enum-1} implies the second property.
\end{proof}

\begin{proofofthm}{\ref{thm:knap-2}}
According to Lemma \ref{lem:Knap-Enum-2}, we combine the new enumeration method and the previous iterative rounding (Algorithm \ref{Algo-IR-Knap}). Recall the output of Algorithm \ref{Algo-Enum-Knap} is a set of partial solutions: \(X \subseteq 2^{S_1} \times 2^{S_2} \times \cdots \times 2^{S_{T_0}}\). For any \((D_1, D_2, \cdots D_{T_0}) \in X\), we run Algorithm \ref{Algo-IR-Knap} with \((D_1, \cdots D_{T_0})\) as part of the input. We can notice that the proof of Lemma \ref{lem:Knap-3} can also apply to the current situation. Therefore, if all of the output partial solutions correspond to "No Solution" as the result of Algorithm \ref{Algo-IR-Knap}, then we can confirm that there is no $1$-valid solution. Otherwise, we find a $2$-valid solution. By Lemmas \ref{lem:Knap-Enum-1} and \ref{lem:Knap-1}, the complexity of iterative rounding is also polynomial time. Overall, this is an algorithm that can solve the $2$-\LBO\ $d$-dimensional knapsack cover problem for $d = O\left(\sqrt{\frac{\log n}{\log\log W}}\right)$.
\end{proofofthm}

\subsection{A (1+$\epsilon$)-approximation algorithm for \minnormknapcov\ with $d=O(1)$}

In this subsection, we consider the following program:

TODO:
